# Supplementary material for: Finite-Field Cholesky Decomposed Coupled-Cluster Techniques (ff-CD-CC): Theory and Application to Pressure Broadening of Mg by a He Atmosphere and a Strong Magnetic Field
Source: arXiv:2409.20267 source file (2024-09-30)
Supplement: Supplementary file 1 [file SI.pdf]

# **Supporting Information: Finite-Field Cholesky Decomposed Coupled-Cluster Techniques (ff-CD-CC): Theory and Application to Pressure Broadening of Mg by a He Atmosphere and a Strong Magnetic Field**

Simon Blaschke,<sup>\*,†,‡</sup> Marios-Petros Kitsaras,<sup>\*,¶</sup> and Stella Stopkowicz<sup>\*,¶,§</sup>

<sup>†</sup>*Department Chemie, Johannes Gutenberg-Universität Mainz, Duesbergweg 10-14, D-55128  
Mainz, Germany*

<sup>‡</sup>*Fachrichtung Chemie, Universität des Saarlandes, Campus B2.2, D-66123 Saarbrücken,  
Germany*

<sup>¶</sup>*Fachrichtung Chemie, Universität des Saarlandes, D-66123 Saarbrücken, Germany*

<sup>§</sup>*Hylleraas Centre for Quantum Molecular Sciences, Department of Chemistry, University  
of Oslo, P.O. Box 1033, N-0315 Oslo, Norway*

E-mail: [siblasch@uni-mainz.de](mailto:siblasch@uni-mainz.de); [marios.kitsaras@uni-saarland.de](mailto:marios.kitsaras@uni-saarland.de);  
[stella.stopkowicz@uni-saarland.de](mailto:stella.stopkowicz@uni-saarland.de)

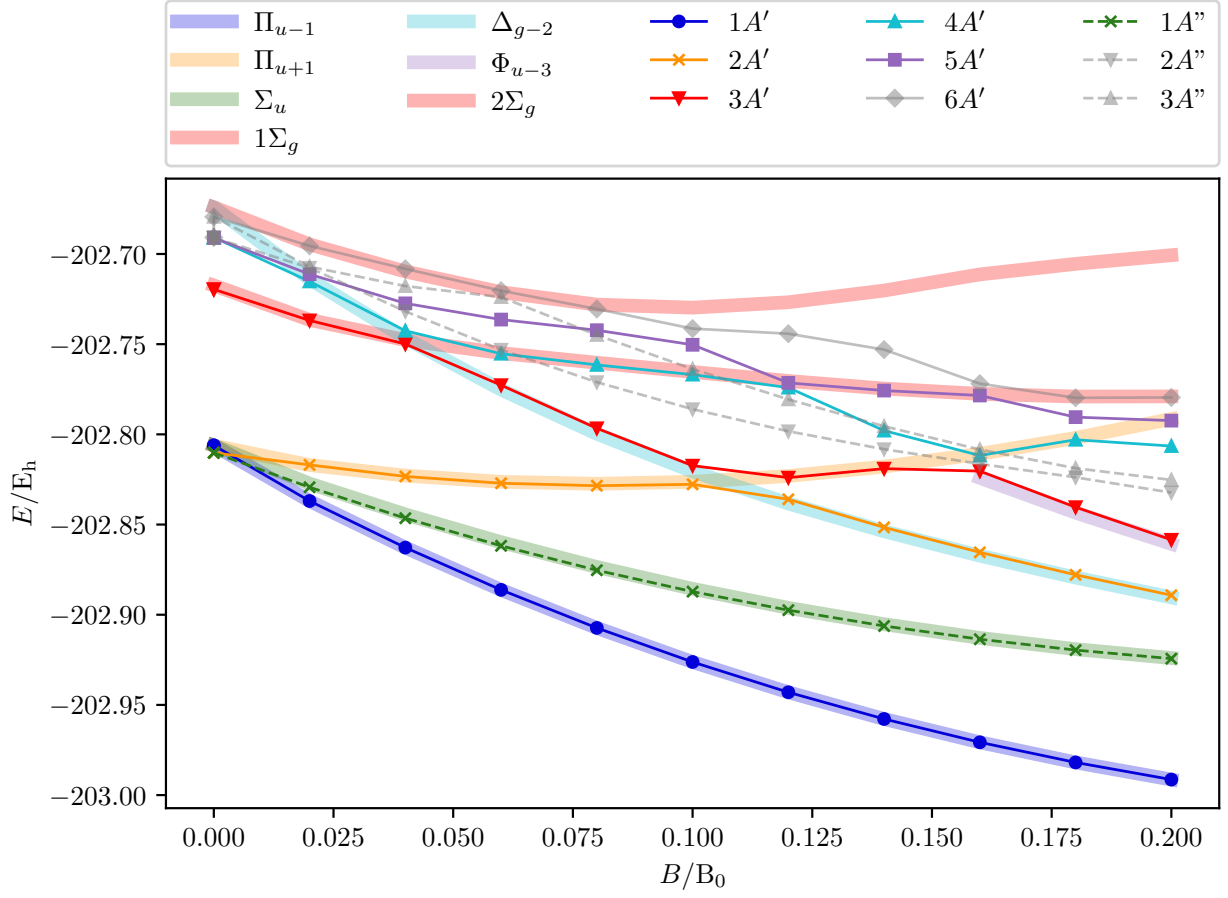

Figure S1: Depiction of the ground and excited states of MgHe in a perpendicular magnetic field ( $C_s$ ). As a guideline of the evolution of the states in the isolated Mg atom ( $SO(3)$ ) the respective states are shown as broad lines. Note that they were shifted by the energy of the helium atom so that the ground state coincides.

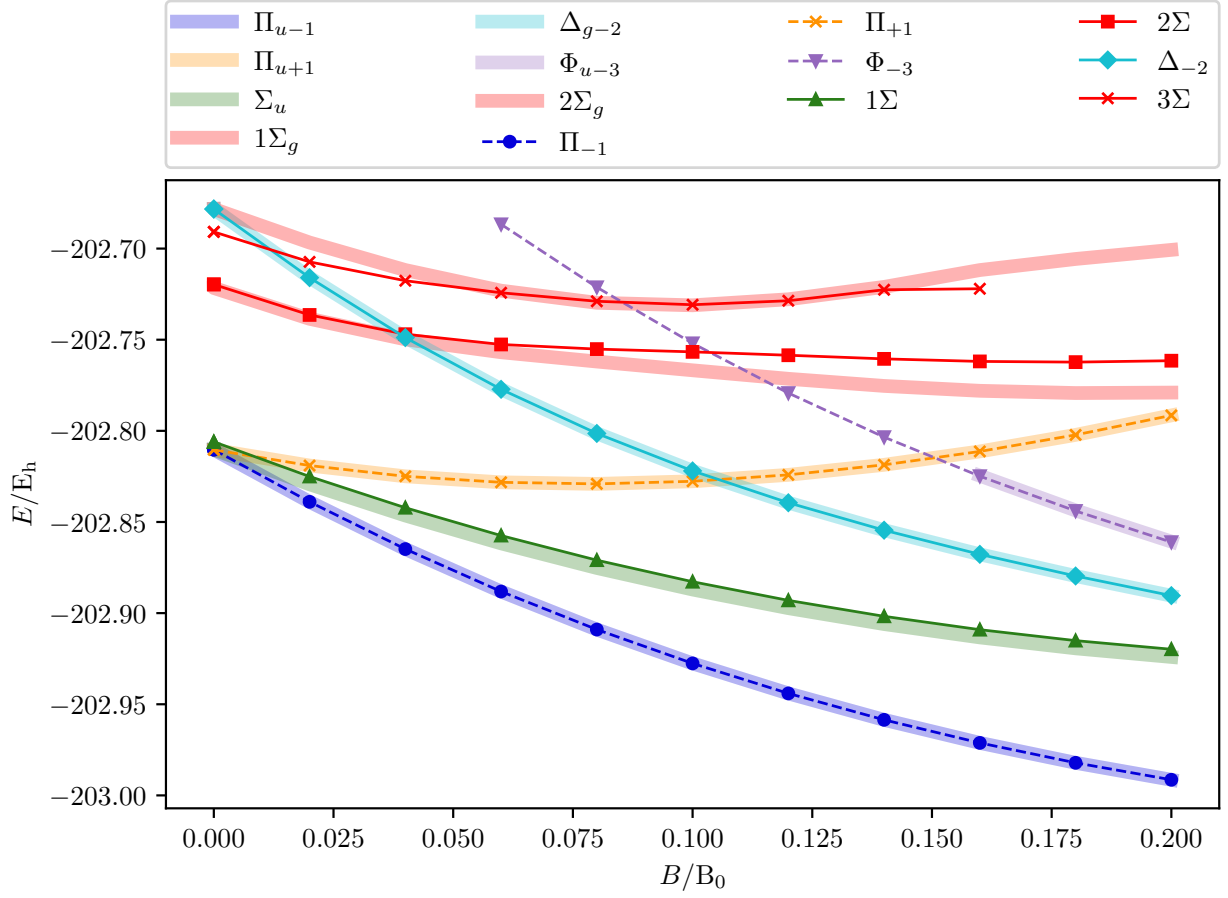

Figure S2: Depiction of the ground and excited states of MgHe in a parallel magnetic field ( $C_\infty$ ). As a guideline of the evolution of the states in the isolated Mg atom ( $SO(3)$ ) the respective states are shown as broad lines. Note that they were shifted by the energy of the helium atom so that the ground state coincides.

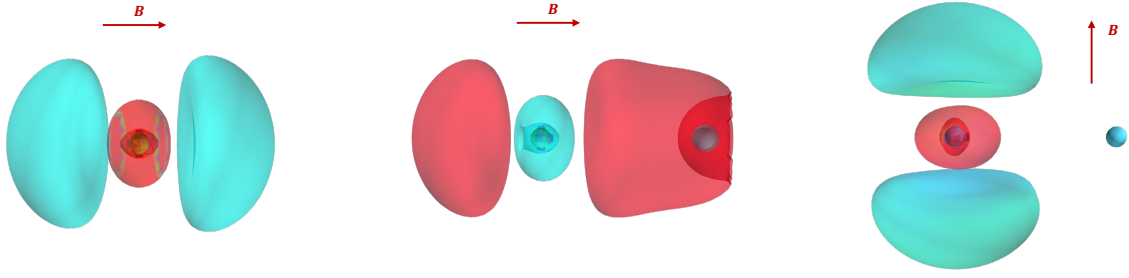

Figure S3: Depiction of the HOMO (4s in the field-free case) of the final state for the  $^3P$  to  $^3S$  transition of the Mg triplet atom (left) in a magnetic field and for MgHe with the magnetic field parallel (center) and perpendicular (right) to the bond axis. Calculated at  $B=0.1 B_0$  as an isosurface plot of  $0.015 a_0^{-3}$ .

Table S1: EOM-CCSD excitation energy  $E_{\text{exc}}$  of the MgHe dimer at  $3.5 \text{ \AA}$  bond distance. The basis set on Mg was chosen to be unc-aug-cc-pCVQZ while the basis on He was varied. The difference in the transition wavelength  $\Delta\lambda$  with respect to the d-aug-cc-pVQZ is given additionally.

| Basis on He       | $E_{\text{exc}}/E_{\text{h}}$ | $\Delta E_{\text{exc}}/E_{\text{h}}$ | $\Delta\lambda/\text{\AA}$ |
|-------------------|-------------------------------|--------------------------------------|----------------------------|
| unc-6-31G         | $9.097\,78 \times 10^{-2}$    | $3.1 \times 10^{-4}$                 | 16.95                      |
| unc-cc-pVDZ       | $9.093\,17 \times 10^{-2}$    | $2.6 \times 10^{-4}$                 | 14.41                      |
| unc-aug-cc-pVDZ   | $9.073\,52 \times 10^{-2}$    | $6.4 \times 10^{-5}$                 | 3.55                       |
| unc-aug-cc-pVTZ   | $9.069\,67 \times 10^{-2}$    | $2.6 \times 10^{-5}$                 | 1.42                       |
| unc-aug-cc-pVQZ   | $9.068\,80 \times 10^{-2}$    | $1.7 \times 10^{-5}$                 | 0.94                       |
| unc-d-aug-cc-pVQZ | $9.067\,11 \times 10^{-2}$    | 0.00                                 | 0.00                       |

Table S2: Mean error of the ff-CD-HF energy, ff-CD-CCSD/CC2 correlation energy and the ff-CD-EOM-CCSD/CC2 excitation energy as a function of the Cholesky parameter  $\delta$ . The convergence criteria for HF, CCSD as well as EOM were set to  $10^{-7}$ .

| $\delta$ | $\Delta E_{\text{HF}}/E_{\text{h}}$ | $\Delta E_{\text{CCSD}}/E_{\text{h}}$ | $\Delta E_{\text{EOM-CCSD}}/E_{\text{h}}$ | $\Delta E_{\text{CC2}}/E_{\text{h}}$ | $\Delta E_{\text{EOM-CC2}}/E_{\text{h}}$ |
|----------|-------------------------------------|---------------------------------------|-------------------------------------------|--------------------------------------|------------------------------------------|
| 1        | $3.7 \times 10^{-2}$                | $2.9 \times 10^{-2}$                  | $2.1 \times 10^{-2}$                      | $2.3 \times 10^{-2}$                 | $1.2 \times 10^{-2}$                     |
| 2        | $9.0 \times 10^{-4}$                | $2.5 \times 10^{-4}$                  | $1.9 \times 10^{-4}$                      | $5.2 \times 10^{-4}$                 | $2.2 \times 10^{-4}$                     |
| 3        | $1.8 \times 10^{-5}$                | $6.7 \times 10^{-6}$                  | $6.3 \times 10^{-6}$                      | $2.1 \times 10^{-5}$                 | $5.8 \times 10^{-6}$                     |
| 4        | $1.6 \times 10^{-6}$                | $2.9 \times 10^{-7}$                  | $5.2 \times 10^{-7}$                      | $9.5 \times 10^{-7}$                 | $4.0 \times 10^{-7}$                     |
| 5        | $6.4 \times 10^{-7}$                | $9.0 \times 10^{-8}$                  | $6.5 \times 10^{-8}$                      | $1.8 \times 10^{-7}$                 | $5.7 \times 10^{-8}$                     |
| 6        | $4.7 \times 10^{-8}$                | $8.6 \times 10^{-9}$                  | $1.4 \times 10^{-8}$                      | $1.6 \times 10^{-8}$                 | $1.2 \times 10^{-8}$                     |
| 7        | $1.3 \times 10^{-8}$                | $3.5 \times 10^{-9}$                  | $2.0 \times 10^{-9}$                      | $4.2 \times 10^{-9}$                 | $3.4 \times 10^{-9}$                     |
| 8        | $9.3 \times 10^{-10}$               | $2.6 \times 10^{-9}$                  | $6.4 \times 10^{-10}$                     | $3.0 \times 10^{-9}$                 | $2.5 \times 10^{-9}$                     |
| 9        | $5.3 \times 10^{-11}$               | $2.6 \times 10^{-9}$                  | $3.6 \times 10^{-10}$                     | $3.0 \times 10^{-9}$                 | $2.3 \times 10^{-9}$                     |
| 10       | 0.0                                 | $2.6 \times 10^{-9}$                  | $3.4 \times 10^{-10}$                     | $3.0 \times 10^{-9}$                 | $2.3 \times 10^{-9}$                     |

Table S3: The transition wavelength  $\lambda$  ( $^3\Pi \rightarrow ^3\Sigma^+$ ) as well as the total initial state energy  $E_{\text{tot}}$  as a function of the Mg-He distance  $R$ . Calculated with CD-CCSD ( $\delta = 5$ ) using the unc-aug-cc-pCVQZ basis for Mg and the unc-aug-cc-pVDZ basis for He.

| $R/\text{\AA}$ | $\lambda/\text{\AA}$ | $E_{\text{tot}}/E_{\text{h}}$ |
|----------------|----------------------|-------------------------------|
| 2.00           | 5196.55              | -202.803197                   |
| 2.50           | 5104.26              | -202.808283                   |
| 3.00           | 5040.01              | -202.809948                   |
| 3.50           | 5024.26              | -202.810382                   |
| 4.00           | 5034.37              | -202.810435                   |
| 4.50           | 5054.82              | -202.810408                   |
| 5.00           | 5076.51              | -202.810375                   |
| 5.50           | 5094.98              | -202.810353                   |
| 6.00           | 5108.79              | -202.810341                   |
| 6.50           | 5118.24              | -202.810334                   |
| 7.00           | 5124.27              | -202.810330                   |
| 7.50           | 5127.92              | -202.810328                   |
| 8.00           | 5130.04              | -202.810327                   |
| 8.50           | 5131.22              | -202.810326                   |
| 9.00           | 5131.85              | -202.810325                   |
| 9.50           | 5132.17              | -202.810325                   |
| 10.00          | 5132.32              | -202.810325                   |
| 10.50          | 5132.38              | -202.810325                   |
| 11.00          | 5132.40              | -202.810324                   |
| 11.50          | 5132.40              | -202.810324                   |
| 12.00          | 5132.40              | -202.810324                   |
| 12.50          | 5132.39              | -202.810324                   |
| 13.00          | 5132.38              | -202.810324                   |
| 13.50          | 5132.38              | -202.810324                   |
| 14.00          | 5132.37              | -202.810324                   |
| 14.50          | 5132.37              | -202.810324                   |
| 15.00          | 5132.37              | -202.810324                   |

Table S4: Total energy  $E_{\text{tot}}$  of the initial and first two final states of the MgHe triplet dimer without an external magnetic field and within an finite magnetic field of  $0.05 B_0$  oriented parallel and perpendicular with respect to the Mg-He axis. The calculations were performed at the unc-aug-cc-pVTZ/CC3 level of theory.

| $B = 0$        |                                  |                                  |                                  |
|----------------|----------------------------------|----------------------------------|----------------------------------|
| $R/\text{\AA}$ | $E_{\text{tot}}(^3\Sigma^+)/E_h$ | $E_{\text{tot}}(^3\Pi_{-1})/E_h$ | $E_{\text{tot}}(^3\Pi_{+1})/E_h$ |
| 3.0            | -202.621464                      | -202.631647                      | -202.631647                      |
| 3.5            | -202.627884                      | -202.632085                      | -202.632085                      |
| 4.0            | -202.630494                      | -202.632140                      | -202.632140                      |
| 4.5            | -202.631507                      | -202.632121                      | -202.632121                      |
| 5.0            | -202.631881                      | -202.632097                      | -202.632097                      |
| 5.5            | -202.632011                      | -202.632079                      | -202.632079                      |
| 6.0            | -202.632052                      | -202.632068                      | -202.632068                      |
| 6.5            | -202.632062                      | -202.632062                      | -202.632062                      |
| 7.0            | -202.632064                      | -202.632058                      | -202.632058                      |
| 7.5            | -202.632063                      | -202.632056                      | -202.632056                      |
| 8.0            | -202.632061                      | -202.632055                      | -202.632055                      |
| $B \parallel$  |                                  |                                  |                                  |
| $R/\text{\AA}$ | $E_{\text{tot}}(^3\Sigma)/E_h$   | $E_{\text{tot}}(^3\Pi_{-1})/E_h$ | $E_{\text{tot}}(^3\Pi_{+1})/E_h$ |
| 3.0            | -202.665333                      | -202.698023                      | -202.648026                      |
| 3.5            | -202.671842                      | -202.698480                      | -202.648483                      |
| 4.0            | -202.674479                      | -202.698543                      | -202.648545                      |
| 4.5            | -202.675498                      | -202.698527                      | -202.648529                      |
| 5.0            | -202.675872                      | -202.698505                      | -202.648507                      |
| 5.5            | -202.676001                      | -202.698488                      | -202.648490                      |
| 6.0            | -202.676041                      | -202.698477                      | -202.648479                      |
| 6.5            | -202.676052                      | -202.698471                      | -202.648473                      |
| 7.0            | -202.676053                      | -202.698467                      | -202.648469                      |
| 7.5            | -202.676052                      | -202.698465                      | -202.648467                      |
| 8.0            | -202.676050                      | -202.698464                      | -202.648466                      |
| $B \perp$      |                                  |                                  |                                  |
| $R/\text{\AA}$ | $E_{\text{tot}}(^3A')/E_h$       | $E_{\text{tot}}(^3A'')/E_h$      | $E_{\text{tot}}(^3A')/E_h$       |
| 3.00           | -202.693170                      | -202.675735                      | -202.644368                      |
| 3.50           | -202.696482                      | -202.676114                      | -202.647151                      |
| 4.00           | -202.697802                      | -202.676144                      | -202.648083                      |
| 4.50           | -202.698275                      | -202.676116                      | -202.648380                      |
| 5.00           | -202.698427                      | -202.676089                      | -                                |
| 5.50           | -202.698467                      | -202.676071                      | -202.648481                      |
| 6.00           | -202.698473                      | -202.676061                      | -202.648479                      |
| 6.50           | -202.698471                      | -202.676055                      | -202.648474                      |
| 7.00           | -202.698468                      | -202.676051                      | -202.648470                      |
| 7.50           | -202.698466                      | -202.676050                      | -202.648468                      |
| 8.00           | -202.698464                      | -202.676048                      | -202.648466                      |

Table S5: The counterpoise corrected CCSD interaction energy of the initial state of the MgHe triplet dimer as a function of the external magnetic field strength in a parallel orientation respectively. The calculations were performed using the unc-aug-cc-pCVQZ basis for Mg and the unc-aug-cc-pVDZ basis for He.

| $R/\text{\AA}$ | $B = 0.0 \text{ B}_0$<br>$E_{\text{int}}/E_h$ | $B = 0.05 \text{ B}_0$<br>$E_{\text{int}}/E_h$ | $B = 0.10 \text{ B}_0$<br>$E_{\text{int}}/E_h$ | $B = 0.15 \text{ B}_0$<br>$E_{\text{int}}/E_h$ | $B = 0.20 \text{ B}_0$<br>$E_{\text{int}}/E_h$ |
|----------------|-----------------------------------------------|------------------------------------------------|------------------------------------------------|------------------------------------------------|------------------------------------------------|
| 3.0            | $5.300 \times 10^{-4}$                        | $5.508 \times 10^{-4}$                         | $5.960 \times 10^{-4}$                         | $6.562 \times 10^{-4}$                         | $7.271 \times 10^{-4}$                         |
| 3.5            | $2.016 \times 10^{-5}$                        | $2.891 \times 10^{-5}$                         | $4.669 \times 10^{-5}$                         | $6.869 \times 10^{-5}$                         | $9.371 \times 10^{-5}$                         |
| 3.6            | $-1.458 \times 10^{-5}$                       | $-7.147 \times 10^{-6}$                        | $7.775 \times 10^{-6}$                         | $2.591 \times 10^{-5}$                         | $4.630 \times 10^{-5}$                         |
| 3.7            | $-3.782 \times 10^{-5}$                       | $-3.148 \times 10^{-5}$                        | $-1.889 \times 10^{-5}$                        | $-3.865 \times 10^{-6}$                        | $1.279 \times 10^{-5}$                         |
| 3.8            | $-5.249 \times 10^{-5}$                       | $-4.705 \times 10^{-5}$                        | $-3.637 \times 10^{-5}$                        | $-2.387 \times 10^{-5}$                        | $-1.023 \times 10^{-5}$                        |
| 3.9            | $-6.087 \times 10^{-5}$                       | $-5.618 \times 10^{-5}$                        | $-4.708 \times 10^{-5}$                        | $-3.662 \times 10^{-5}$                        | $-2.541 \times 10^{-5}$                        |
| 4.0            | $-6.473 \times 10^{-5}$                       | $-6.068 \times 10^{-5}$                        | $-5.288 \times 10^{-5}$                        | $-4.409 \times 10^{-5}$                        | $-3.484 \times 10^{-5}$                        |
| 4.1            | $-6.543 \times 10^{-5}$                       | $-6.191 \times 10^{-5}$                        | $-5.520 \times 10^{-5}$                        | $-4.777 \times 10^{-5}$                        | $-4.012 \times 10^{-5}$                        |
| 4.2            | $-6.399 \times 10^{-5}$                       | $-6.092 \times 10^{-5}$                        | $-5.512 \times 10^{-5}$                        | $-4.881 \times 10^{-5}$                        | $-4.245 \times 10^{-5}$                        |
| 4.3            | $-6.116 \times 10^{-5}$                       | $-5.847 \times 10^{-5}$                        | $-5.344 \times 10^{-5}$                        | $-4.805 \times 10^{-5}$                        | $-4.274 \times 10^{-5}$                        |
| 4.4            | $-5.748 \times 10^{-5}$                       | $-5.513 \times 10^{-5}$                        | $-5.075 \times 10^{-5}$                        | $-4.613 \times 10^{-5}$                        | $-4.168 \times 10^{-5}$                        |
| 4.5            | $-5.337 \times 10^{-5}$                       | $-5.130 \times 10^{-5}$                        | $-4.747 \times 10^{-5}$                        | $-4.350 \times 10^{-5}$                        | $-3.975 \times 10^{-5}$                        |
| 4.6            | $-4.909 \times 10^{-5}$                       | $-4.727 \times 10^{-5}$                        | $-4.391 \times 10^{-5}$                        | $-4.049 \times 10^{-5}$                        | $-3.730 \times 10^{-5}$                        |
| 4.7            | $-4.484 \times 10^{-5}$                       | $-4.323 \times 10^{-5}$                        | $-4.028 \times 10^{-5}$                        | $-3.731 \times 10^{-5}$                        | $-3.460 \times 10^{-5}$                        |
| 4.8            | $-4.074 \times 10^{-5}$                       | $-3.931 \times 10^{-5}$                        | $-3.672 \times 10^{-5}$                        | $-3.414 \times 10^{-5}$                        | $-3.182 \times 10^{-5}$                        |
| 4.9            | $-3.687 \times 10^{-5}$                       | $-3.561 \times 10^{-5}$                        | $-3.332 \times 10^{-5}$                        | $-3.107 \times 10^{-5}$                        | $-2.907 \times 10^{-5}$                        |
| 5.0            | $-3.327 \times 10^{-5}$                       | $-3.215 \times 10^{-5}$                        | $-3.014 \times 10^{-5}$                        | $-2.816 \times 10^{-5}$                        | $-2.643 \times 10^{-5}$                        |
| 5.5            | $-1.956 \times 10^{-5}$                       | $-1.893 \times 10^{-5}$                        | $-1.782 \times 10^{-5}$                        | $-1.677 \times 10^{-5}$                        | $-1.587 \times 10^{-5}$                        |
| 6.0            | $-1.159 \times 10^{-5}$                       | $-1.122 \times 10^{-5}$                        | $-1.059 \times 10^{-5}$                        | $-9.987 \times 10^{-6}$                        | $-9.475 \times 10^{-6}$                        |
| 6.5            | $-7.070 \times 10^{-6}$                       | $-6.846 \times 10^{-6}$                        | $-6.466 \times 10^{-6}$                        | $-6.103 \times 10^{-6}$                        | $-5.792 \times 10^{-6}$                        |
| 7.0            | $-4.465 \times 10^{-6}$                       | $-4.323 \times 10^{-6}$                        | $-4.082 \times 10^{-6}$                        | $-3.851 \times 10^{-6}$                        | $-3.652 \times 10^{-6}$                        |
| 7.5            | $-2.916 \times 10^{-6}$                       | $-2.822 \times 10^{-6}$                        | $-2.663 \times 10^{-6}$                        | $-2.509 \times 10^{-6}$                        | $-2.375 \times 10^{-6}$                        |
| 8.0            | $-1.962 \times 10^{-6}$                       | $-1.897 \times 10^{-6}$                        | $-1.789 \times 10^{-6}$                        | $-1.682 \times 10^{-6}$                        | $-1.590 \times 10^{-6}$                        |

Table S6: The counterpoise corrected CCSD interaction energy of the initial state of the MgHe triplet dimer as a function of the external magnetic field strength in a perpendicular orientation respectively. The calculations were performed using the unc-aug-cc-pCVQZ basis for Mg and the unc-aug-cc-pVDZ basis for He.

| $R/\text{\AA}$ | $B = 0.0 \text{ B}_0$<br>$E_{\text{int}}/E_{\text{h}}$ | $B = 0.05 \text{ B}_0$<br>$E_{\text{int}}/E_{\text{h}}$ | $B = 0.10 \text{ B}_0$<br>$E_{\text{int}}/E_{\text{h}}$ | $B = 0.15 \text{ B}_0$<br>$E_{\text{int}}/E_{\text{h}}$ | $B = 0.20 \text{ B}_0$<br>$E_{\text{int}}/E_{\text{h}}$ |
|----------------|--------------------------------------------------------|---------------------------------------------------------|---------------------------------------------------------|---------------------------------------------------------|---------------------------------------------------------|
| 3.0            | $5.300 \times 10^{-4}$                                 | $5.421 \times 10^{-3}$                                  | $4.623 \times 10^{-3}$                                  | $3.078 \times 10^{-3}$                                  | $1.588 \times 10^{-3}$                                  |
| 3.5            | $2.016 \times 10^{-5}$                                 | $2.048 \times 10^{-3}$                                  | $1.424 \times 10^{-3}$                                  | $6.667 \times 10^{-4}$                                  | $1.132 \times 10^{-4}$                                  |
| 3.6            | $-1.458 \times 10^{-5}$                                | $1.664 \times 10^{-3}$                                  | $1.100 \times 10^{-3}$                                  | $4.606 \times 10^{-4}$                                  | $2.193 \times 10^{-5}$                                  |
| 3.7            | $-3.782 \times 10^{-5}$                                | $1.347 \times 10^{-3}$                                  | $8.423 \times 10^{-4}$                                  | $3.067 \times 10^{-4}$                                  | $-3.680 \times 10^{-5}$                                 |
| 3.8            | $-5.249 \times 10^{-5}$                                | $1.085 \times 10^{-3}$                                  | $6.384 \times 10^{-4}$                                  | $1.936 \times 10^{-4}$                                  | $-7.215 \times 10^{-5}$                                 |
| 3.9            | $-6.087 \times 10^{-5}$                                | $8.712 \times 10^{-4}$                                  | $4.782 \times 10^{-4}$                                  | $1.118 \times 10^{-4}$                                  | $-9.112 \times 10^{-5}$                                 |
| 4.0            | $-6.473 \times 10^{-5}$                                | $6.962 \times 10^{-4}$                                  | $3.533 \times 10^{-4}$                                  | $5.383 \times 10^{-5}$                                  | $-9.894 \times 10^{-5}$                                 |
| 4.1            | $-6.543 \times 10^{-5}$                                | $5.538 \times 10^{-4}$                                  | $2.566 \times 10^{-4}$                                  | $1.384 \times 10^{-5}$                                  | $-9.947 \times 10^{-5}$                                 |
| 4.2            | $-6.399 \times 10^{-5}$                                | $4.383 \times 10^{-4}$                                  | $1.823 \times 10^{-4}$                                  | $-1.284 \times 10^{-5}$                                 | $-9.547 \times 10^{-5}$                                 |
| 4.3            | $-6.116 \times 10^{-5}$                                | $3.449 \times 10^{-4}$                                  | $1.259 \times 10^{-4}$                                  | $-2.980 \times 10^{-5}$                                 | $-8.890 \times 10^{-5}$                                 |
| 4.4            | $-5.748 \times 10^{-5}$                                | $2.697 \times 10^{-4}$                                  | $8.331 \times 10^{-5}$                                  | $-3.978 \times 10^{-5}$                                 | $-8.107 \times 10^{-5}$                                 |
| 4.5            | $-5.337 \times 10^{-5}$                                | $2.094 \times 10^{-4}$                                  | $5.163 \times 10^{-5}$                                  | $-4.484 \times 10^{-5}$                                 | $-7.285 \times 10^{-5}$                                 |
| 4.6            | $-4.909 \times 10^{-5}$                                | $1.612 \times 10^{-4}$                                  | $2.838 \times 10^{-5}$                                  | $-4.655 \times 10^{-5}$                                 | $-6.480 \times 10^{-5}$                                 |
| 4.7            | $-4.484 \times 10^{-5}$                                | $1.228 \times 10^{-4}$                                  | $1.159 \times 10^{-5}$                                  | $-4.602 \times 10^{-5}$                                 | $-5.722 \times 10^{-5}$                                 |
| 4.8            | $-4.074 \times 10^{-5}$                                | $9.245 \times 10^{-5}$                                  | $-2.602 \times 10^{-7}$                                 | $-4.408 \times 10^{-5}$                                 | $-5.029 \times 10^{-5}$                                 |
| 4.9            | $-3.687 \times 10^{-5}$                                | $6.849 \times 10^{-5}$                                  | $-8.386 \times 10^{-6}$                                 | $-4.131 \times 10^{-5}$                                 | $-4.407 \times 10^{-5}$                                 |
| 5.0            | $-3.327 \times 10^{-5}$                                | $4.970 \times 10^{-5}$                                  | $-1.373 \times 10^{-5}$                                 | $-3.813 \times 10^{-5}$                                 | $-3.857 \times 10^{-5}$                                 |
| 5.1            | -                                                      | $3.505 \times 10^{-5}$                                  | $-1.701 \times 10^{-5}$                                 | $-3.479 \times 10^{-5}$                                 | $-3.374 \times 10^{-5}$                                 |
| 5.2            | -                                                      | $2.372 \times 10^{-5}$                                  | $-1.880 \times 10^{-5}$                                 | $-3.150 \times 10^{-5}$                                 | $-2.954 \times 10^{-5}$                                 |
| 5.3            | -                                                      | $1.503 \times 10^{-5}$                                  | $-1.953 \times 10^{-5}$                                 | $-2.835 \times 10^{-5}$                                 | $-2.589 \times 10^{-5}$                                 |
| 5.4            | -                                                      | $8.431 \times 10^{-6}$                                  | $-1.950 \times 10^{-5}$                                 | $-2.541 \times 10^{-5}$                                 | $-2.274 \times 10^{-5}$                                 |
| 5.5            | $-1.956 \times 10^{-5}$                                | $3.478 \times 10^{-6}$                                  | $-1.897 \times 10^{-5}$                                 | $-2.272 \times 10^{-5}$                                 | $-2.001 \times 10^{-5}$                                 |
| 5.6            | -                                                      | $-1.791 \times 10^{-7}$                                 | $-1.811 \times 10^{-5}$                                 | $-2.028 \times 10^{-5}$                                 | $-1.764 \times 10^{-5}$                                 |
| 5.7            | -                                                      | $-2.825 \times 10^{-6}$                                 | $-1.706 \times 10^{-5}$                                 | $-1.809 \times 10^{-5}$                                 | $-1.560 \times 10^{-5}$                                 |
| 5.8            | -                                                      | $-4.687 \times 10^{-6}$                                 | $-1.591 \times 10^{-5}$                                 | $-1.613 \times 10^{-5}$                                 | $-1.383 \times 10^{-5}$                                 |
| 5.9            | -                                                      | $-5.944 \times 10^{-6}$                                 | $-1.472 \times 10^{-5}$                                 | $-1.440 \times 10^{-5}$                                 | $-1.229 \times 10^{-5}$                                 |
| 6.0            | $-1.159 \times 10^{-5}$                                | $-6.740 \times 10^{-6}$                                 | $-1.355 \times 10^{-5}$                                 | $-1.286 \times 10^{-5}$                                 | $-1.095 \times 10^{-5}$                                 |
| 6.1            | -                                                      | $-7.188 \times 10^{-6}$                                 | $-1.241 \times 10^{-5}$                                 | $-1.150 \times 10^{-5}$                                 | $-9.781 \times 10^{-6}$                                 |
| 6.2            | -                                                      | $-7.376 \times 10^{-6}$                                 | $-1.134 \times 10^{-5}$                                 | $-1.030 \times 10^{-5}$                                 | $-8.757 \times 10^{-6}$                                 |
| 6.3            | -                                                      | $-7.373 \times 10^{-6}$                                 | $-1.033 \times 10^{-5}$                                 | $-9.239 \times 10^{-6}$                                 | $-7.859 \times 10^{-6}$                                 |
| 6.4            | -                                                      | $-7.234 \times 10^{-6}$                                 | $-9.399 \times 10^{-6}$                                 | $-8.302 \times 10^{-6}$                                 | $-7.068 \times 10^{-6}$                                 |
| 6.5            | $-7.070 \times 10^{-6}$                                | $-6.999 \times 10^{-6}$                                 | $-8.544 \times 10^{-6}$                                 | $-7.474 \times 10^{-6}$                                 | $-6.370 \times 10^{-6}$                                 |
| 7.0            | $-4.465 \times 10^{-6}$                                | $-5.271 \times 10^{-6}$                                 | $-5.307 \times 10^{-6}$                                 | $-4.538 \times 10^{-6}$                                 | $-3.897 \times 10^{-6}$                                 |
| 7.5            | $-2.916 \times 10^{-6}$                                | $-3.640 \times 10^{-6}$                                 | $-3.364 \times 10^{-6}$                                 | $-2.873 \times 10^{-6}$                                 | $-2.482 \times 10^{-6}$                                 |
| 8.0            | $-1.962 \times 10^{-6}$                                | $-2.464 \times 10^{-6}$                                 | $-2.196 \times 10^{-6}$                                 | $-1.884 \times 10^{-6}$                                 | $-1.635 \times 10^{-6}$                                 |

Table S7: Transition wavelength  $\lambda$  of the three former  $P$ -states as a function of the magnetic field strength  $B$ . Three cases are distinguished. The isolated Mg atom is used as a reference ( $C_{\infty h}$ , solid) and is compared with the MgHe triplet dimer at the equilibrium distance in the parallel ( $C_{\infty}$ , dotted) or perpendicular ( $C_s$ , dashed) magnetic field. Calculated with CD-CCSD ( $\delta = 5$ ) using the unc-aug-cc-pCVQZ basis for Mg and the unc-aug-cc-pVDZ basis for He.

| Mg atom |                               |                                  |                               |
|---------|-------------------------------|----------------------------------|-------------------------------|
| $B/B_0$ | $\lambda(^3\Pi_u)/\text{\AA}$ | $\lambda(^3\Sigma_u)/\text{\AA}$ | $\lambda(^3\Pi_u)/\text{\AA}$ |
| 0.00    | 5132.4                        | 5132.4                           | 5132.4                        |
| 0.02    | 4539.7                        | 5021.7                           | 5662.3                        |
| 0.04    | 3962.0                        | 4716.5                           | 6065.8                        |
| 0.05    | 3703.6                        | 4532.4                           | 6229.5                        |
| 0.06    | 3472.9                        | 4348.4                           | 6388.4                        |
| 0.08    | 3100.6                        | 4025.6                           | 6791.9                        |
| 0.10    | 2835.0                        | 3790.7                           | 7485.5                        |
| 0.12    | 2641.3                        | 3623.3                           | 8651.0                        |
| 0.14    | 2488.6                        | 3489.5                           | 10532.6                       |
| 0.15    | 2422.0                        | 3428.5                           | 11895.3                       |
| 0.16    | 2360.0                        | 3369.5                           | 13704.1                       |
| 0.18    | 2247.2                        | 3254.9                           | 19852.1                       |
| 0.20    | 2146.1                        | 3143.1                           | 36412.4                       |

  

| MgHe $B \perp$ |                            |                             |                            |
|----------------|----------------------------|-----------------------------|----------------------------|
| $B/B_0$        | $\lambda(^3A')/\text{\AA}$ | $\lambda(^3A'')/\text{\AA}$ | $\lambda(^3A')/\text{\AA}$ |
| 0.00           | 5037.0                     | 5116.8                      | 5037.0                     |
| 0.05           | 3674.1                     | 4459.2                      | 6126.9                     |
| 0.10           | 2841.3                     | 3790.4                      | 7488.6                     |
| 0.15           | 2424.9                     | 3431.1                      | 11886.1                    |
| 0.20           | 2148.0                     | 3146.9                      | 36562.7                    |

  

| MgHe $B \parallel$ |                                  |                                |                                  |
|--------------------|----------------------------------|--------------------------------|----------------------------------|
| $B/B_0$            | $\lambda(^3\Pi_{-1})/\text{\AA}$ | $\lambda(^3\Sigma)/\text{\AA}$ | $\lambda(^3\Pi_{+1})/\text{\AA}$ |
| 0.00               | 5037.0                           | 5116.8                         | 5037.0                           |
| 0.05               | 3620.3                           | 4471.0                         | 5997.3                           |
| 0.10               | 2713.1                           | 3616.1                         | 6691.8                           |
| 0.15               | 2299.1                           | 3217.7                         | 9421.4                           |
| 0.20               | 2043.9                           | 2952.8                         | 19693.7                          |

Table S8: Shift in the excitation energies  $\Delta E_{\text{exc}}$  induced by the helium atom for the three former  $P$ -states of the MgHe triplet dimer at the equilibrium distance in a parallel ( $C_{\infty}$ , dotted) or perpendicular ( $C_s$ , dashed) magnetic field compared to the isolated Mg atom. For the absolute excitation energies also see tab. S7.

| $B/B_0$ | MgHe $B \perp$                        |                                        |                                       | MgHe $B \parallel$                          |                                           |                                             |
|---------|---------------------------------------|----------------------------------------|---------------------------------------|---------------------------------------------|-------------------------------------------|---------------------------------------------|
|         | $^3A'$<br>$\Delta E_{\text{exc}}/E_h$ | $^3A''$<br>$\Delta E_{\text{exc}}/E_h$ | $^3A'$<br>$\Delta E_{\text{exc}}/E_h$ | $^3\Pi_{-1}$<br>$\Delta E_{\text{exc}}/E_h$ | $^3\Sigma$<br>$\Delta E_{\text{exc}}/E_h$ | $^3\Pi_{+1}$<br>$\Delta E_{\text{exc}}/E_h$ |
| 0.00    | $-1.681 \times 10^{-3}$               | $-2.701 \times 10^{-4}$                | $-1.681 \times 10^{-3}$               | $-1.681 \times 10^{-3}$                     | $-2.701 \times 10^{-4}$                   | $-1.681 \times 10^{-3}$                     |
| 0.05    | $-9.882 \times 10^{-4}$               | $-1.650 \times 10^{-3}$                | $-1.225 \times 10^{-3}$               | $-2.833 \times 10^{-3}$                     | $-1.382 \times 10^{-3}$                   | $-2.834 \times 10^{-3}$                     |
| 0.10    | $3.617 \times 10^{-4}$                | $-1.065 \times 10^{-5}$                | $2.545 \times 10^{-5}$                | $-7.222 \times 10^{-3}$                     | $-5.809 \times 10^{-3}$                   | $-7.223 \times 10^{-3}$                     |
| 0.15    | $2.255 \times 10^{-4}$                | $9.926 \times 10^{-5}$                 | $-2.964 \times 10^{-5}$               | $-1.006 \times 10^{-2}$                     | $-8.712 \times 10^{-3}$                   | $-1.006 \times 10^{-2}$                     |
| 0.20    | $1.811 \times 10^{-4}$                | $1.793 \times 10^{-4}$                 | $5.148 \times 10^{-5}$                | $-1.063 \times 10^{-2}$                     | $-9.343 \times 10^{-3}$                   | $-1.063 \times 10^{-2}$                     |

Table S9: Shift in the transition wavelength and energies  $\Delta\lambda = \lambda(\rho \rightarrow 0) - \lambda(\rho)$  ( $\Delta E_{\text{exc}} = E_{\text{exc}}(\rho \rightarrow 0) - E_{\text{exc}}(\rho)$ ) on CD-CCSD ( $\delta = 5$ ) level of the Mg triplet transition as a function of the helium density  $\rho$  of the MgHe<sub>12</sub> ( $C_{3h}$ ) atmospheric model system in a magnetic field of 3000 T oriented along the  $C_3$  axis. Employing the unc-aug-cc-pCVQZ on Mg and the unc-aug-cc-pVDZ basis on He.

| $n(\text{He})/\text{cm}^{-3}$ | $B = 0$<br>$\Delta\lambda/\text{\AA}$ | $\Delta\lambda(E')/\text{\AA}$  | $B \neq 0$<br>$\Delta\lambda(A')/\text{\AA}$ | $\Delta E_{\text{exc}}(E')/\text{\AA}$ |
|-------------------------------|---------------------------------------|---------------------------------|----------------------------------------------|----------------------------------------|
| $1.94 \times 10^{21}$         | 6.23                                  | 4.70                            | 5.38                                         | 6.25                                   |
| $4.12 \times 10^{21}$         | 100.62                                | 81.60                           | 93.31                                        | 108.26                                 |
| $6.55 \times 10^{21}$         | 305.95                                | 254.96                          | 290.91                                       | 336.78                                 |
| $1.13 \times 10^{22}$         | 760.85                                | 649.64                          | 737.79                                       | 849.94                                 |
| $2.21 \times 10^{22}$         | 1072.02                               | 936.95                          | 1065.32                                      | 1232.01                                |
| $3.30 \times 10^{22}$         | 498.78                                | 422.63                          | 504.33                                       | 628.18                                 |
| $n(\text{He})/\text{cm}^{-3}$ | $\Delta E_{\text{exc}}/E_h$           | $\Delta E_{\text{exc}}(E')/E_h$ | $\Delta E_{\text{exc}}(A')/E_h$              | $\Delta E_{\text{exc}}(E')/E_h$        |
| $1.94 \times 10^{21}$         | $1.079 \times 10^{-4}$                | $9.468 \times 10^{-5}$          | $9.468 \times 10^{-5}$                       | $9.483 \times 10^{-5}$                 |
| $4.12 \times 10^{21}$         | $1.776 \times 10^{-3}$                | $1.672 \times 10^{-3}$          | $1.671 \times 10^{-3}$                       | $1.674 \times 10^{-3}$                 |
| $6.55 \times 10^{21}$         | $5.631 \times 10^{-3}$                | $5.424 \times 10^{-3}$          | $5.425 \times 10^{-3}$                       | $5.439 \times 10^{-3}$                 |
| $1.13 \times 10^{22}$         | $1.546 \times 10^{-2}$                | $1.515 \times 10^{-2}$          | $1.517 \times 10^{-2}$                       | $1.525 \times 10^{-2}$                 |
| $2.21 \times 10^{22}$         | $2.345 \times 10^{-2}$                | $2.349 \times 10^{-2}$          | $2.369 \times 10^{-2}$                       | $2.409 \times 10^{-2}$                 |
| $3.30 \times 10^{22}$         | $9.561 \times 10^{-3}$                | $9.338 \times 10^{-3}$          | $9.843 \times 10^{-3}$                       | $1.075 \times 10^{-2}$                 |

Table S10: Shift in the transition wavelength and energies  $\Delta\lambda = \lambda(\rho \rightarrow 0) - \lambda(\rho)$  ( $\Delta E_{\text{exc}} = E_{\text{exc}}(\rho \rightarrow 0) - E_{\text{exc}}(\rho)$ ) on CD-CCSD ( $\delta = 5$ ) level of the Mg triplet transition as a function of the helium density  $\rho$  of the MgHe<sub>12</sub> ( $C_{3h}$ ) atmospheric model system in a magnetic field of 30000 T oriented along the  $C_3$  axis. Employing the unc-aug-cc-pCVQZ on Mg and the unc-aug-cc-pVDZ basis on He.

| $n(\text{He})/\text{cm}^{-3}$ | $B = 0$<br>$\Delta\lambda/\text{\AA}$ | $\Delta\lambda(E')/\text{\AA}$  | $B \neq 0$<br>$\Delta\lambda(A')/\text{\AA}$ | $\Delta E_{\text{exc}}(E')/\text{\AA}$ |
|-------------------------------|---------------------------------------|---------------------------------|----------------------------------------------|----------------------------------------|
| $1.94 \times 10^{21}$         | 6.23                                  | -0.45                           | -0.82                                        | -5.76                                  |
| $4.12 \times 10^{21}$         | 100.62                                | -1.33                           | -2.49                                        | -17.13                                 |
| $6.55 \times 10^{21}$         | 305.95                                | 7.97                            | 14.86                                        | 103.53                                 |
| $1.13 \times 10^{22}$         | 760.85                                | 60.97                           | 111.48                                       | 774.58                                 |
| $2.21 \times 10^{22}$         | 1072.02                               | 182.98                          | 324.98                                       | 2288.37                                |
| $3.30 \times 10^{22}$         | 498.78                                | 261.29                          | 474.09                                       | 2404.29                                |
| $n(\text{He})/\text{cm}^{-3}$ | $\Delta E_{\text{exc}}/E_h$           | $\Delta E_{\text{exc}}(E')/E_h$ | $\Delta E_{\text{exc}}(A')/E_h$              | $\Delta E_{\text{exc}}(E')/E_h$        |
| $1.94 \times 10^{21}$         | $1.079 \times 10^{-4}$                | $-3.073 \times 10^{-5}$         | $-2.949 \times 10^{-5}$                      | $-3.059 \times 10^{-5}$                |
| $4.12 \times 10^{21}$         | $1.776 \times 10^{-3}$                | $-9.098 \times 10^{-5}$         | $-8.897 \times 10^{-5}$                      | $-9.083 \times 10^{-5}$                |
| $6.55 \times 10^{21}$         | $5.631 \times 10^{-3}$                | $5.477 \times 10^{-4}$          | $5.338 \times 10^{-4}$                       | $5.561 \times 10^{-4}$                 |
| $1.13 \times 10^{22}$         | $1.546 \times 10^{-2}$                | $4.279 \times 10^{-3}$          | $4.117 \times 10^{-3}$                       | $4.489 \times 10^{-3}$                 |
| $2.21 \times 10^{22}$         | $2.345 \times 10^{-2}$                | $1.350 \times 10^{-2}$          | $1.279 \times 10^{-2}$                       | $1.614 \times 10^{-2}$                 |
| $3.30 \times 10^{22}$         | $9.561 \times 10^{-3}$                | $1.992 \times 10^{-2}$          | $1.956 \times 10^{-2}$                       | $1.725 \times 10^{-2}$                 |

Table S11: Transition wavelength and transition dipole moments  $|\mu_{IJ}|^2$  on CD-CCSD ( $\delta = 5$ ) level of the Mg triplet transition as a function of the helium density  $\rho$  of the MgHe<sub>12</sub> ( $C_{3h}$ ) atmospheric model system in a magnetic field of 3000 T oriented along the  $C_3$  axis. Employing the unc-aug-cc-pCVQZ on Mg and the unc-aug-cc-pVDZ basis on He.

| $n(\text{He})/\text{cm}^{-3}$ | $\Delta\lambda(E')/\text{\AA}$ | $ \mu_{IJ} ^2/e^2a_0^2$ | $\Delta\lambda(A')/\text{\AA}$ | $ \mu_{IJ} ^2/e^2a_0^2$ | $\Delta\lambda(E')/\text{\AA}$ | $ \mu_{IJ} ^2/e^2a_0^2$ |
|-------------------------------|--------------------------------|-------------------------|--------------------------------|-------------------------|--------------------------------|-------------------------|
| $1.94 \times 10^{21}$         | 4335.88                        | 0.00                    | 4587.39                        | 0.00                    | 4855.77                        | 0.05                    |
| $4.12 \times 10^{21}$         | 4753.81                        | 2.34                    | 5086.34                        | 2.37                    | 5477.70                        | 2.31                    |
| $6.55 \times 10^{21}$         | 4676.90                        | 2.37                    | 4998.41                        | 2.41                    | 5375.69                        | 2.36                    |
| $1.13 \times 10^{22}$         | 4503.55                        | 2.36                    | 4800.81                        | 2.39                    | 5147.17                        | 2.35                    |
| $2.21 \times 10^{22}$         | 4108.86                        | 2.07                    | 4353.93                        | 2.10                    | 4634.01                        | 2.09                    |
| $3.30 \times 10^{22}$         | 3821.56                        | 0.77                    | 4026.41                        | 0.80                    | 4251.93                        | 0.82                    |

Table S12: EOM-CC2 excitation energy of the MgHe<sub>12</sub> and MgHe<sub>56</sub> cluster using a lattice constant of 3 Å which equates to a density of  $6.5 \times 10^{21}$  atoms/cm<sup>3</sup>. A magnetic field of 3000 T was oriented along the  $C_3$  axis. The basis set on Mg was chosen to be unc-aug-cc-pCVQZ while the basis on He was unc-aug-cc-pVDZ.

|                    |                               | $E'$                          |                      | $A'$                          |                      | $E'$                          |                      |
|--------------------|-------------------------------|-------------------------------|----------------------|-------------------------------|----------------------|-------------------------------|----------------------|
|                    | $n(\text{He})/\text{cm}^{-3}$ | $E_{\text{exc}}/E_{\text{h}}$ | $\lambda/\text{\AA}$ | $E_{\text{exc}}/E_{\text{h}}$ | $\lambda/\text{\AA}$ | $E_{\text{exc}}/E_{\text{h}}$ | $\lambda/\text{\AA}$ |
| MgHe <sub>12</sub> | $6.5 \times 10^{21}$          | 0.101694                      | 4482.82              | 0.094735                      | 4812.14              | 0.090007                      | 5064.90              |
| MgHe <sub>56</sub> | $6.5 \times 10^{21}$          | 0.101820                      | 4477.29              | 0.094861                      | 4805.75              | 0.090132                      | 5057.89              |
| Difference         |                               |                               | 5.54                 |                               | 6.39                 |                               | 7.01                 |

Table S13: Equilibrium geometries of the MgHe dimer in the triplet state as a function of the magnetic field strength.

| $B/B_0$ | parallel                   | perpendicular              |
|---------|----------------------------|----------------------------|
|         | $R_{\text{eq}}/\text{\AA}$ | $R_{\text{eq}}/\text{\AA}$ |
| 0       | 4.0744                     | 4.0744                     |
| 0.05    | 4.0961                     | 6.2495                     |
| 0.1     | 4.1414                     | 5.3340                     |
| 0.15    | 4.2000                     | 4.6164                     |
| 0.2     | 4.2677                     | 4.0531                     |

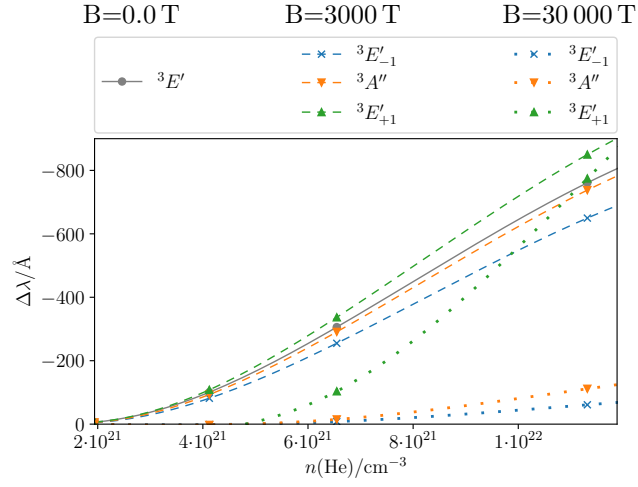

Figure S4: Shift in the transition wavelength  $\Delta\lambda$  with respect atomic transition for triplet Mg as a function of the helium density  $\rho$  of the  $\text{MgHe}_{12}$  ( $C_{3h}$ ) atmospheric model system for the field-free case (grey full curve) and in a magnetic fields of 3000 T (dashed curves) as well as 30 000 T (dotted curves) oriented along the  $C_3$  axis. Calculated at the CD-CCSD ( $\delta = 5$ ) level employing the unc-aug-cc-pCVQZ on Mg and the unc-aug-cc-pVDZ basis on He.

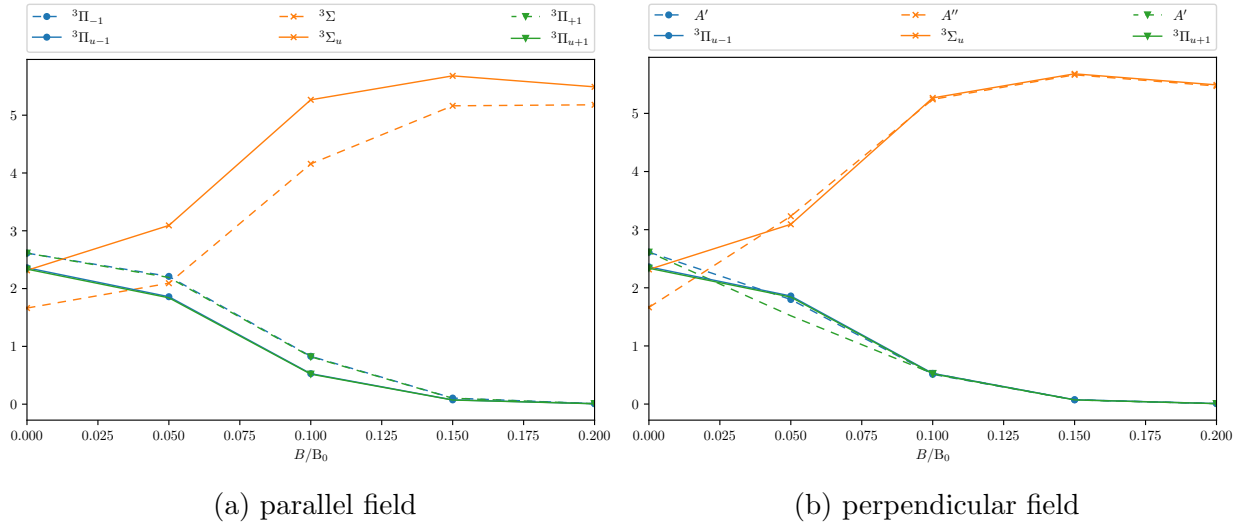

Figure S5: Evolution of the transition-dipole moment of the transitions in the triplet  $\text{MgHe}$  dimer as a function of the magnetic field strength (dashed lines). As reference the transition-dipole moment of an isolated atom is plotted (full lines). The calculations were performed using ff-CD-CCSD and the unc-aug-cc-pCVQZ basis for Mg and the unc-aug-cc-pVDZ basis for He.

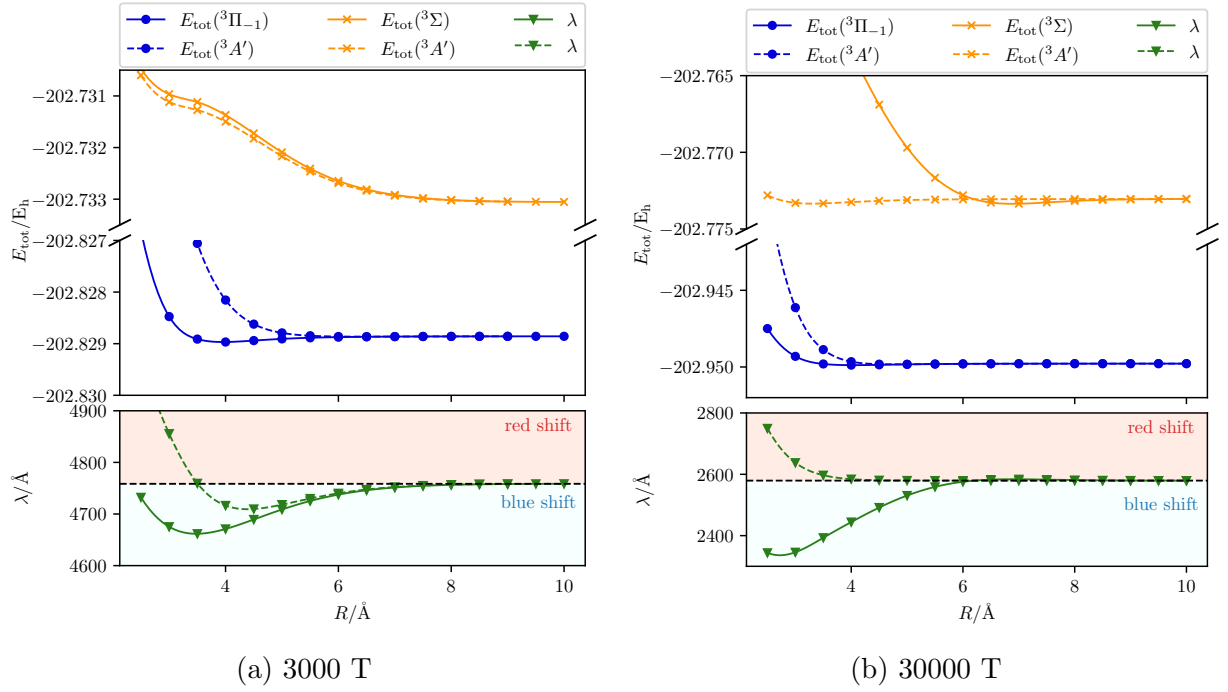

Figure S6: Transition wavelengths  $\lambda$  in a parallel ( $^3\Pi_{-1} \rightarrow ^3\Sigma$ , full lines) and perpendicular orientation ( $^3A' \rightarrow ^3A'$ , dashed lines) in a magnetic field of 3000 T and 30000 T as well as the total initial-state energy  $E_{\text{tot}}$  as a function of the Mg-He distance  $R$ . Calculated with CD-CCSD ( $\delta = 5$ ) using the unc-aug-cc-pCVQZ basis for Mg and the unc-aug-cc-pVDZ basis for He.

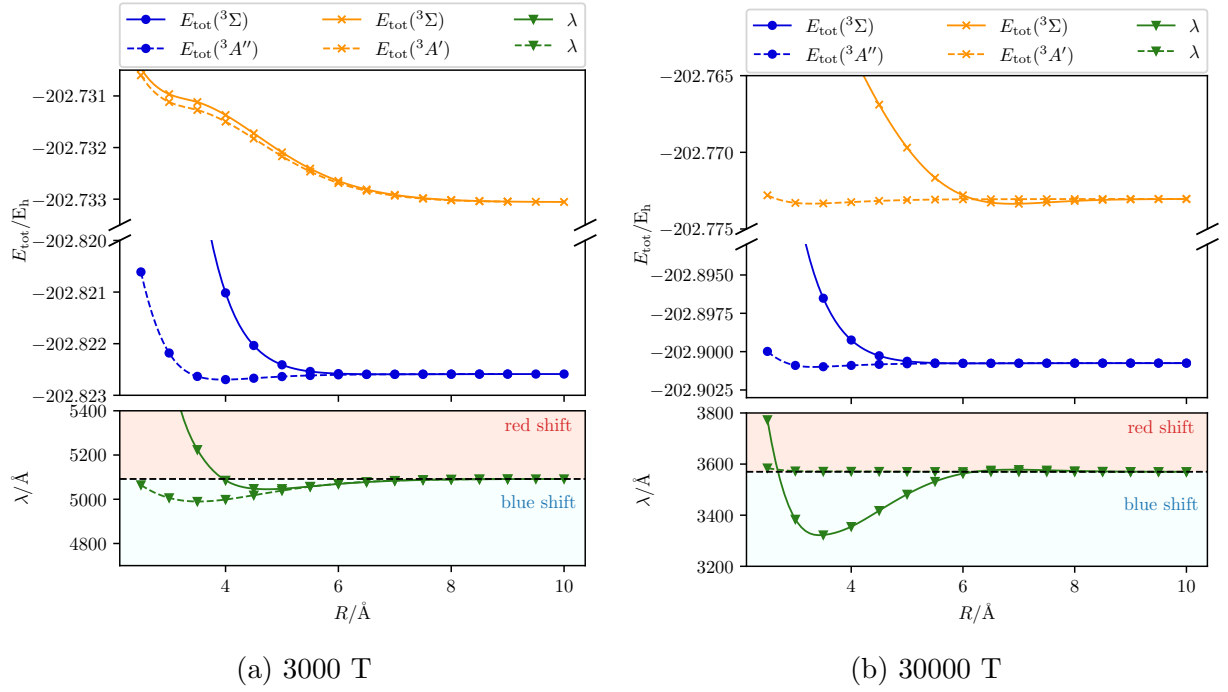

Figure S7: Transition wavelengths  $\lambda$  in a parallel ( $^3\Sigma \rightarrow ^3\Sigma$ , full lines) and perpendicular orientation ( $^3A'' \rightarrow ^3A'$ , dashed lines) in a magnetic field of 3000 T and 30000 T as well as the total initial-state energy  $E_{\text{tot}}$  as a function of the Mg-He distance  $R$ . Calculated with CD-CCSD ( $\delta = 5$ ) using the unc-aug-cc-pCVQZ basis for Mg and the unc-aug-cc-pVDZ basis for He.
